# Supplementary material for: Imagine Before Concentration: Diffusion-Guided Registers Enhance Partially Relevant Video Retrieval
Source: arXiv:2604.03653 source file (2026-04-04)
Supplement: Supplementary file 1 [file appendix_main.tex]

\documentclass[10pt,twocolumn,letterpaper]{article}

\usepackage{cvpr}

% Import additional packages in the preamble file, before hyperref
\input{preamble}
\input{command}

% If you wish to avoid re-using figure, table, and equation numbers from
% the main paper, please uncomment the following and change the numbers
% appropriately.
\setcounter{figure}{6}
\setcounter{table}{3}
\setcounter{equation}{17}

\begin{document}
\clearpage

%%%%%%%%% TITLE - PLEASE UPDATE
\title{Imagine Before Concentration: Diffusion-Guided Registers \\ Enhance Partially Relevant Video Retrieval}
\maketitlesupplementary

\thispagestyle{empty}
\appendix

\input{appendix_sections/Method}

%%%%%%%%% REFERENCES
{
    \small
    \bibliographystyle{ieeenat_fullname}
    \bibliography{main}
}

\end{document}
